# Supplementary material for: Excitons in solid molecular hydrogen from quantum Monte Carlo
Source: arXiv:2610.39894 source file (2026-10-29)
Supplement: Supplementary file 1 [file suppmat.tex]

\documentclass[10pt,aps,showpacs,superscriptaddress,floatfix,nofootinbib]{revtex4-2}


\pdfoutput=1
\usepackage[utf8]{inputenc}
\usepackage[english]{babel}
\usepackage[T1]{fontenc}
\usepackage{csquotes}
% \usepackage{physics}
\usepackage{amsmath,amsfonts}
\usepackage{enumitem}

\usepackage[dvipsnames]{xcolor}
\usepackage[colorlinks=true]{hyperref}
\usepackage[capitalise]{cleveref}

\usepackage{listings}

\usepackage{multirow}
\usepackage{graphicx}
\usepackage{subcaption}
\usepackage{tikz}

\graphicspath{{figures/}}

\usepackage{bm} 

\usepackage[normalem]{ulem} 
% \newcommand{\edit}[1]{{\color{red}#1}}
% \newcommand{\todelete}[1]{{\color{red}\sout{#1}}}
\DeclareRobustCommand{\edit}[1]{{\color{red}#1}}
\newcommand{\mh}[1]{{\color{blue}mh: #1}} 
\definecolor{ao(english)}{rgb}{0.0, 0.5, 0.0}
\newcommand{\sm}[1]{{\color{ao(english)}#1}} 
\DeclareRobustCommand{\todelete}[1]{}

\hypersetup{hidelinks}

\begin{document}
\title{Supplementary Material: Excitons in solid molecular hydrogen from quantum Monte Carlo}

\author{Edgar Josué Landinez Borda}
\altaffiliation{Present address: Forschungszentrum Jülich GmbH, Wilhelm-Johnen-Straße, 52428 Jülich, Germany}
\affiliation{MESA+ Institute for Nanotechnology, University of Twente, P.O. Box 217, 7500 AE Enschede, The Netherlands}
\author{Ravindra Shinde}
\affiliation{MESA+ Institute for Nanotechnology, University of Twente, P.O. Box 217, 7500 AE Enschede, The Netherlands}
\author{Claudia Filippi}
\affiliation{MESA+ Institute for Nanotechnology, University of Twente, P.O. Box 217, 7500 AE Enschede, The Netherlands}
\author{Markus Holzmann}
\affiliation{Univ. Grenoble Alpes, CNRS; LPMMC, 38000 Grenoble, France}
\author{Saverio Moroni}
\affiliation{CNR-IOM DEMOCRITOS, Istituto Officina dei Materiali and SISSA Scuola Internazionale Superiore di Studi Avanzati, Via Bonomea 265, I-34136 Trieste, Italy}
\maketitle

\section*{Supplementary Material}


In this Section we display additional results for the 
excitation-induced density difference $\Delta\rho({\bf r})$ (Figures~\ref{fig:drho-a1-a5}-\ref{fig:drho-c16-c19}) and transition dipole moment ${\boldsymbol\mu}_{01}$ (Figures~\ref{fig:tdma}-{\ref{fig:tdmc}).
We also list in Table~\ref{table:os} results for the 
oscillator strength $2/3\langle{\boldsymbol\mu}_{01}\cdot{\boldsymbol\mu}_{01}(E_1-E_0)\rangle$, where $\langle\cdot\rangle$ indicates average over the nuclear configurations, and
$E_1-E_0$ is the neutral gap.

% 5gpa 1-5 %%%%%%%%%%%%%%%%%%%%%%%%%%%%%%%%%%%%%%%%%%%%%%%%%%%%%%%%%%%%%%%%%%%%%%%%%%%%%%%%%%%

\begin{figure*}[h]

\hspace{-1.0cm}
\begin{subfigure}{0.17\textwidth}
\captionsetup{labelformat=empty}
\caption{{\em 1CSF0}}
\includegraphics[width=3.0cm,height=3.0cm]{figures/c1-5gpa-hf.pdf}
\label{hf_a1}
\end{subfigure}
\begin{subfigure}{0.17\textwidth}
\captionsetup{labelformat=empty}
\caption{DMC {\em J1CSF}}
\includegraphics[width=3.0cm,height=3.0cm]{figures/c1-5gpa-jcsf.pdf}
\label{vmc_a1}
\end{subfigure}
\begin{subfigure}{0.17\textwidth}
\captionsetup{labelformat=empty}
\caption{TDDFT}
\includegraphics[width=3.0cm,height=3.0cm]{figures/c1-5gpa-tddft.pdf}
\label{pbe0_a1}
\end{subfigure}
\begin{subfigure}{0.17\textwidth}
\captionsetup{labelformat=empty}
\caption{BSE}
\includegraphics[width=3.0cm,height=3.0cm]{figures/c1-5gpa-bse.pdf}
\label{bse_a1}
\end{subfigure}
\begin{subfigure}{0.17\textwidth}
\captionsetup{labelformat=empty}
\caption{{\em CIS0}}
\includegraphics[width=3.0cm,height=3.0cm]{figures/c1-5gpa-cis.pdf}
\label{cis_a1}
\end{subfigure}
\begin{subfigure}{0.17\textwidth}
\captionsetup{labelformat=empty}
\caption{DMC {\em JCIS}}
%\includegraphics[width=3.0cm,height=3.0cm]{figures/c1-5gpa-jcis.pdf}
\begin{tikzpicture}
\node at (0,0){\includegraphics[width=3.0cm,height=3.0cm]{figures/c1-5gpa-jcis.pdf}};
\draw[] node at (2,0){\bf a1};
\end{tikzpicture}
\label{dmc_a1}
\end{subfigure}

\hspace{-1.0cm}
\begin{subfigure}{0.17\textwidth}
\includegraphics[width=3.0cm,height=3.0cm]{figures/c2-5gpa-hf.pdf}
\label{hf_a2}
\end{subfigure}
\begin{subfigure}{0.17\textwidth}
\includegraphics[width=3.0cm,height=3.0cm]{figures/c2-5gpa-jcsf.pdf}
\label{vmc_a2}
\end{subfigure}
\begin{subfigure}{0.17\textwidth}
\includegraphics[width=3.0cm,height=3.0cm]{figures/c2-5gpa-tddft.pdf}
\label{pbe0_a2}
\end{subfigure}
\begin{subfigure}{0.17\textwidth}
\includegraphics[width=3.0cm,height=3.0cm]{figures/c2-5gpa-bse.pdf}
\label{bse_a2}
\end{subfigure}
\begin{subfigure}{0.17\textwidth}
\includegraphics[width=3.0cm,height=3.0cm]{figures/c2-5gpa-cis.pdf}
\label{cis_a2}
\end{subfigure}
\begin{subfigure}{0.17\textwidth}
%\includegraphics[width=3.0cm,height=3.0cm]{figures/c2-5gpa-jcis.pdf}
\begin{tikzpicture}
\node at (0,0){\includegraphics[width=3.0cm,height=3.0cm]{figures/c2-5gpa-jcis.pdf}};
\draw[] node at (2,0){\bf a2};
\end{tikzpicture}
\label{dmc_a2}
\end{subfigure}

\hspace{-1.0cm}
\begin{subfigure}{0.17\textwidth}
\includegraphics[width=3.0cm,height=3.0cm]{figures/c3-5gpa-hf.pdf}
\label{hf_a3}
\end{subfigure}
\begin{subfigure}{0.17\textwidth}
\includegraphics[width=3.0cm,height=3.0cm]{figures/c3-5gpa-jcsf.pdf}
\label{vmc_a3}
\end{subfigure}
\begin{subfigure}{0.17\textwidth}
\includegraphics[width=3.0cm,height=3.0cm]{figures/c3-5gpa-tddft.pdf}
\label{pbe0_a3}
\end{subfigure}
\begin{subfigure}{0.17\textwidth}
\includegraphics[width=3.0cm,height=3.0cm]{figures/c3-5gpa-bse.pdf}
\label{bse_a3}
\end{subfigure}
\begin{subfigure}{0.17\textwidth}
\includegraphics[width=3.0cm,height=3.0cm]{figures/c3-5gpa-cis.pdf}
\label{cis_a3}
\end{subfigure}
\begin{subfigure}{0.17\textwidth}
%\includegraphics[width=3.0cm,height=3.0cm]{figures/c3-5gpa-jcis.pdf}
\begin{tikzpicture}
\node at (0,0){\includegraphics[width=3.0cm,height=3.0cm]{figures/c3-5gpa-jcis.pdf}};
\draw[] node at (2,0){\bf a3};
\end{tikzpicture}
\label{dmc_a3}
\end{subfigure}

\hspace{-1.0cm}
\begin{subfigure}{0.17\textwidth}
\includegraphics[width=3.0cm,height=3.0cm]{figures/c4-5gpa-hf.pdf}
\label{hf_a4}
\end{subfigure}
\begin{subfigure}{0.17\textwidth}
\includegraphics[width=3.0cm,height=3.0cm]{figures/c4-5gpa-jcsf.pdf}
\label{vmc_a4}
\end{subfigure}
\begin{subfigure}{0.17\textwidth}
\includegraphics[width=3.0cm,height=3.0cm]{figures/c4-5gpa-tddft.pdf}
\label{pbe0_a4}
\end{subfigure}
\begin{subfigure}{0.17\textwidth}
\includegraphics[width=3.0cm,height=3.0cm]{figures/c4-5gpa-bse.pdf}
\label{bse_a4}
\end{subfigure}
\begin{subfigure}{0.17\textwidth}
\includegraphics[width=3.0cm,height=3.0cm]{figures/c4-5gpa-cis.pdf}
\label{cis_a4}
\end{subfigure}
\begin{subfigure}{0.17\textwidth}
%\includegraphics[width=3.0cm,height=3.0cm]{figures/c4-5gpa-jcis.pdf}
\begin{tikzpicture}
\node at (0,0){\includegraphics[width=3.0cm,height=3.0cm]{figures/c4-5gpa-jcis.pdf}};
\draw[] node at (2,0){\bf a4};
\end{tikzpicture}
\label{dmc_a4}
\end{subfigure}

\hspace{-1.0cm}
\begin{subfigure}{0.17\textwidth}
\includegraphics[width=3.0cm,height=3.0cm]{figures/c5-5gpa-hf.pdf}
\label{hf_a5}
\end{subfigure}
\begin{subfigure}{0.17\textwidth}
\includegraphics[width=3.0cm,height=3.0cm]{figures/c5-5gpa-jcsf.pdf}
\label{vmc_a5}
\end{subfigure}
\begin{subfigure}{0.17\textwidth}
\includegraphics[width=3.0cm,height=3.0cm]{figures/c5-5gpa-tddft.pdf}
\label{pbe0_a5}
\end{subfigure}
\begin{subfigure}{0.17\textwidth}
\includegraphics[width=3.0cm,height=3.0cm]{figures/c5-5gpa-bse.pdf}
\label{bse_a5}
\end{subfigure}
\begin{subfigure}{0.17\textwidth}
\includegraphics[width=3.0cm,height=3.0cm]{figures/c5-5gpa-cis.pdf}
\label{cis_a5}
\end{subfigure}
\begin{subfigure}{0.17\textwidth}
%\includegraphics[width=3.0cm,height=3.0cm]{figures/c5-5gpa-jcis.pdf}
\begin{tikzpicture}
\node at (0,0){\includegraphics[width=3.0cm,height=3.0cm]{figures/c5-5gpa-jcis.pdf}};
\draw[] node at (2,0){\bf a5};
\end{tikzpicture}
\label{dmc_a5}
\end{subfigure}

\caption{Excitation-induced density difference, $\Delta\rho({\bf r})$, for
nuclear configurations {\bf a1}--{\bf a5} at $\rho/\rho_0=3.15$.
}
\label{fig:drho-a1-a5}
\end{figure*}

% 5gpa 6-10 %%%%%%%%%%%%%%%%%%%%%%%%%%%%%%%%%%%%%%%%%%%%%%%%%%%%%%%%%%%%%%%%%%%%%%%%%%%%%%%%%%

\begin{figure*}[h]

\hspace{-1.0cm}
\begin{subfigure}{0.17\textwidth}
\captionsetup{labelformat=empty}
\caption{{\em 1CSF0}}
\includegraphics[width=3.0cm,height=3.0cm]{figures/c6-5gpa-hf.pdf}
\label{hf_a6}
\end{subfigure}
\begin{subfigure}{0.17\textwidth}
\captionsetup{labelformat=empty}
\caption{DMC {\em J1CSF}}
\includegraphics[width=3.0cm,height=3.0cm]{figures/c6-5gpa-jcsf.pdf}
\label{vmc_a6}
\end{subfigure}
\begin{subfigure}{0.17\textwidth}
\captionsetup{labelformat=empty}
\caption{TDDFT}
\includegraphics[width=3.0cm,height=3.0cm]{figures/c6-5gpa-tddft.pdf}
\label{pbe0_a6}
\end{subfigure}
\begin{subfigure}{0.17\textwidth}
\captionsetup{labelformat=empty}
\caption{BSE}
\includegraphics[width=3.0cm,height=3.0cm]{figures/c6-5gpa-bse.pdf}
\label{bse_a6}
\end{subfigure}
\begin{subfigure}{0.17\textwidth}
\captionsetup{labelformat=empty}
\caption{{\em CIS0}}
\includegraphics[width=3.0cm,height=3.0cm]{figures/c6-5gpa-cis.pdf}
\label{cis_a6}
\end{subfigure}
\begin{subfigure}{0.17\textwidth}
\captionsetup{labelformat=empty}
\caption{DMC {\em JCIS}}
%\includegraphics[width=3.0cm,height=3.0cm]{figures/c6-5gpa-jcis.pdf}
\begin{tikzpicture}
\node at (0,0){\includegraphics[width=3.0cm,height=3.0cm]{figures/c6-5gpa-jcis.pdf}};
\draw[] node at (2,0){\bf a6};
\end{tikzpicture}
\label{dmc_a6}
\end{subfigure}

\hspace{-1.0cm}
\begin{subfigure}{0.17\textwidth}
\includegraphics[width=3.0cm,height=3.0cm]{figures/c7-5gpa-hf.pdf}
\label{hf_a7}
\end{subfigure}
\begin{subfigure}{0.17\textwidth}
\includegraphics[width=3.0cm,height=3.0cm]{figures/c7-5gpa-jcsf.pdf}
\label{vmc_a7}
\end{subfigure}
\begin{subfigure}{0.17\textwidth}
\includegraphics[width=3.0cm,height=3.0cm]{figures/c7-5gpa-tddft.pdf}
\label{pbe0_a7}
\end{subfigure}
\begin{subfigure}{0.17\textwidth}
\includegraphics[width=3.0cm,height=3.0cm]{figures/c7-5gpa-bse.pdf}
\label{bse_a7}
\end{subfigure}
\begin{subfigure}{0.17\textwidth}
\includegraphics[width=3.0cm,height=3.0cm]{figures/c7-5gpa-cis.pdf}
\label{cis_a7}
\end{subfigure}
\begin{subfigure}{0.17\textwidth}
%\includegraphics[width=3.0cm,height=3.0cm]{figures/c7-5gpa-jcis.pdf}
\begin{tikzpicture}
\node at (0,0){\includegraphics[width=3.0cm,height=3.0cm]{figures/c7-5gpa-jcis.pdf}};
\draw[] node at (2,0){\bf a7};
\end{tikzpicture}
\label{dmc_a7}
\end{subfigure}

\hspace{-1.0cm}
\begin{subfigure}{0.17\textwidth}
\includegraphics[width=3.0cm,height=3.0cm]{figures/c8-5gpa-hf.pdf}
\label{hf_a8}
\end{subfigure}
\begin{subfigure}{0.17\textwidth}
\includegraphics[width=3.0cm,height=3.0cm]{figures/c8-5gpa-jcsf.pdf}
\label{vmc_a8}
\end{subfigure}
\begin{subfigure}{0.17\textwidth}
\includegraphics[width=3.0cm,height=3.0cm]{figures/c8-5gpa-tddft.pdf}
\label{pbe0_a8}
\end{subfigure}
\begin{subfigure}{0.17\textwidth}
\includegraphics[width=3.0cm,height=3.0cm]{figures/c8-5gpa-bse.pdf}
\label{bse_a8}
\end{subfigure}
\begin{subfigure}{0.17\textwidth}
\includegraphics[width=3.0cm,height=3.0cm]{figures/c8-5gpa-cis.pdf}
\label{cis_a8}
\end{subfigure}
\begin{subfigure}{0.17\textwidth}
%\includegraphics[width=3.0cm,height=3.0cm]{figures/c8-5gpa-jcis.pdf}
\begin{tikzpicture}
\node at (0,0){\includegraphics[width=3.0cm,height=3.0cm]{figures/c8-5gpa-jcis.pdf}};
\draw[] node at (2,0){\bf a8};
\end{tikzpicture}
\label{dmc_a8}
\end{subfigure}

\hspace{-1.0cm}
\begin{subfigure}{0.17\textwidth}
\includegraphics[width=3.0cm,height=3.0cm]{figures/c9-5gpa-hf.pdf}
\label{hf_a9}
\end{subfigure}
\begin{subfigure}{0.17\textwidth}
\includegraphics[width=3.0cm,height=3.0cm]{figures/c9-5gpa-jcsf.pdf}
\label{vmc_a9}
\end{subfigure}
\begin{subfigure}{0.17\textwidth}
\includegraphics[width=3.0cm,height=3.0cm]{figures/c9-5gpa-tddft.pdf}
\label{pbe0_a9}
\end{subfigure}
\begin{subfigure}{0.17\textwidth}
\includegraphics[width=3.0cm,height=3.0cm]{figures/c9-5gpa-bse.pdf}
\label{bse_a9}
\end{subfigure}
\begin{subfigure}{0.17\textwidth}
\includegraphics[width=3.0cm,height=3.0cm]{figures/c9-5gpa-cis.pdf}
\label{cis_a9}
\end{subfigure}
\begin{subfigure}{0.17\textwidth}
%\includegraphics[width=3.0cm,height=3.0cm]{figures/c9-5gpa-jcis.pdf}
\begin{tikzpicture}
\node at (0,0){\includegraphics[width=3.0cm,height=3.0cm]{figures/c9-5gpa-jcis.pdf}};
\draw[] node at (2,0){\bf a9};
\end{tikzpicture}
\label{dmc_a9}
\end{subfigure}

\hspace{-1.0cm}
\begin{subfigure}{0.17\textwidth}
\includegraphics[width=3.0cm,height=3.0cm]{figures/c10-5gpa-hf.pdf}
\label{hf_a10}
\end{subfigure}
\begin{subfigure}{0.17\textwidth}
\includegraphics[width=3.0cm,height=3.0cm]{figures/c10-5gpa-jcsf.pdf}
\label{vmc_a10}
\end{subfigure}
\begin{subfigure}{0.17\textwidth}
\includegraphics[width=3.0cm,height=3.0cm]{figures/c10-5gpa-tddft.pdf}
\label{pbe0_a10}
\end{subfigure}
\begin{subfigure}{0.17\textwidth}
\includegraphics[width=3.0cm,height=3.0cm]{figures/c10-5gpa-bse.pdf}
\label{bse_a10}
\end{subfigure}
\begin{subfigure}{0.17\textwidth}
\includegraphics[width=3.0cm,height=3.0cm]{figures/c10-5gpa-cis.pdf}
\label{cis_a10}
\end{subfigure}
\begin{subfigure}{0.17\textwidth}
%\includegraphics[width=3.0cm,height=3.0cm]{figures/c10-5gpa-jcis.pdf}
\begin{tikzpicture}
\node at (0,0){\includegraphics[width=3.0cm,height=3.0cm]{figures/c10-5gpa-jcis.pdf}};
\draw[] node at (2,0){\bf a10};
\end{tikzpicture}
\label{dmc_a10}
\end{subfigure}

\caption{Excitation-induced density difference, $\Delta\rho({\bf r})$, for
nuclear configurations {\bf a6}--{\bf a10} at $\rho/\rho_0=3.15$.
}
\label{fig:drho-a6-a10}
\end{figure*}


% 10gpa 1-5 %%%%%%%%%%%%%%%%%%%%%%%%%%%%%%%%%%%%%%%%%%%%%%%%%%%%%%%%%%%%%%%%%%%%%%%%%%%%%%%%%%%

\begin{figure*}[h]

\hspace{-1.0cm}
\begin{subfigure}{0.17\textwidth}
\captionsetup{labelformat=empty}
\caption{{\em 1CSF0}}
\includegraphics[width=3.0cm,height=3.0cm]{figures/c1-10gpa-hf.pdf}
\label{hf_b1}
\end{subfigure}
\begin{subfigure}{0.17\textwidth}
\captionsetup{labelformat=empty}
\caption{DMC {\em J1CSF}}
\includegraphics[width=3.0cm,height=3.0cm]{figures/c1-10gpa-jcsf.pdf}
\label{vmc_b1}
\end{subfigure}
\begin{subfigure}{0.17\textwidth}
\captionsetup{labelformat=empty}
\caption{TDDFT}
\includegraphics[width=3.0cm,height=3.0cm]{figures/c1-10gpa-tddft.pdf}
\label{pbe0_b1}
\end{subfigure}
\begin{subfigure}{0.17\textwidth}
\captionsetup{labelformat=empty}
\caption{BSE}
\includegraphics[width=3.0cm,height=3.0cm]{figures/c1-10gpa-bse.pdf}
\label{bse_b1}
\end{subfigure}
\begin{subfigure}{0.17\textwidth}
\captionsetup{labelformat=empty}
\caption{{\em CIS0}}
\includegraphics[width=3.0cm,height=3.0cm]{figures/c1-10gpa-cis.pdf}
\label{cis_b1}
\end{subfigure}
\begin{subfigure}{0.17\textwidth}
\captionsetup{labelformat=empty}
\caption{DMC {\em JCIS}}
%\includegraphics[width=3.0cm,height=3.0cm]{figures/c1-10gpa-jcis.pdf}
\begin{tikzpicture}
\node at (0,0){\includegraphics[width=3.0cm,height=3.0cm]{figures/c1-10gpa-jcis.pdf}};
\draw[] node at (2,0){\bf b1};
\end{tikzpicture}
\label{dmc_b1}
\end{subfigure}

\hspace{-1.0cm}
\begin{subfigure}{0.17\textwidth}
\includegraphics[width=3.0cm,height=3.0cm]{figures/c2-10gpa-hf.pdf}
\label{hf_b2}
\end{subfigure}
\begin{subfigure}{0.17\textwidth}
\includegraphics[width=3.0cm,height=3.0cm]{figures/c2-10gpa-jcsf.pdf}
\label{vmc_b2}
\end{subfigure}
\begin{subfigure}{0.17\textwidth}
\includegraphics[width=3.0cm,height=3.0cm]{figures/c2-10gpa-tddft.pdf}
\label{pbe0_b2}
\end{subfigure}
\begin{subfigure}{0.17\textwidth}
\includegraphics[width=3.0cm,height=3.0cm]{figures/c2-10gpa-bse.pdf}
\label{bse_b2}
\end{subfigure}
\begin{subfigure}{0.17\textwidth}
\includegraphics[width=3.0cm,height=3.0cm]{figures/c2-10gpa-cis.pdf}
\label{cis_b2}
\end{subfigure}
\begin{subfigure}{0.17\textwidth}
%\includegraphics[width=3.0cm,height=3.0cm]{figures/c2-10gpa-jcis.pdf}
\begin{tikzpicture}
\node at (0,0){\includegraphics[width=3.0cm,height=3.0cm]{figures/c2-10gpa-jcis.pdf}};
\draw[] node at (2,0){\bf b2};
\end{tikzpicture}
\label{dmc_b2}
\end{subfigure}

\hspace{-1.0cm}
\begin{subfigure}{0.17\textwidth}
\includegraphics[width=3.0cm,height=3.0cm]{figures/c3-10gpa-hf.pdf}
\label{hf_b3}
\end{subfigure}
\begin{subfigure}{0.17\textwidth}
\includegraphics[width=3.0cm,height=3.0cm]{figures/c3-10gpa-jcsf.pdf}
\label{vmc_b3}
\end{subfigure}
\begin{subfigure}{0.17\textwidth}
\includegraphics[width=3.0cm,height=3.0cm]{figures/c3-10gpa-tddft.pdf}
\label{pbe0_b3}
\end{subfigure}
\begin{subfigure}{0.17\textwidth}
\includegraphics[width=3.0cm,height=3.0cm]{figures/c3-10gpa-bse.pdf}
\label{bse_b3}
\end{subfigure}
\begin{subfigure}{0.17\textwidth}
\includegraphics[width=3.0cm,height=3.0cm]{figures/c3-10gpa-cis.pdf}
\label{cis_b3}
\end{subfigure}
\begin{subfigure}{0.17\textwidth}
%\includegraphics[width=3.0cm,height=3.0cm]{figures/c3-10gpa-jcis.pdf}
\begin{tikzpicture}
\node at (0,0){\includegraphics[width=3.0cm,height=3.0cm]{figures/c3-10gpa-jcis.pdf}};
\draw[] node at (2,0){\bf b3};
\end{tikzpicture}
\label{dmc_b3}
\end{subfigure}

\hspace{-1.0cm}
\begin{subfigure}{0.17\textwidth}
\includegraphics[width=3.0cm,height=3.0cm]{figures/c4-10gpa-hf.pdf}
\label{hf_b4}
\end{subfigure}
\begin{subfigure}{0.17\textwidth}
\includegraphics[width=3.0cm,height=3.0cm]{figures/c4-10gpa-jcsf.pdf}
\label{vmc_b4}
\end{subfigure}
\begin{subfigure}{0.17\textwidth}
\includegraphics[width=3.0cm,height=3.0cm]{figures/c4-10gpa-tddft.pdf}
\label{pbe0_b4}
\end{subfigure}
\begin{subfigure}{0.17\textwidth}
\includegraphics[width=3.0cm,height=3.0cm]{figures/c4-10gpa-bse.pdf}
\label{bse_b4}
\end{subfigure}
\begin{subfigure}{0.17\textwidth}
\includegraphics[width=3.0cm,height=3.0cm]{figures/c4-10gpa-cis.pdf}
\label{cis_b4}
\end{subfigure}
\begin{subfigure}{0.17\textwidth}
%\includegraphics[width=3.0cm,height=3.0cm]{figures/c4-10gpa-jcis.pdf}
\begin{tikzpicture}
\node at (0,0){\includegraphics[width=3.0cm,height=3.0cm]{figures/c4-10gpa-jcis.pdf}};
\draw[] node at (2,0){\bf b4};
\end{tikzpicture}
\label{dmc_b4}
\end{subfigure}

\hspace{-1.0cm}
\begin{subfigure}{0.17\textwidth}
\includegraphics[width=3.0cm,height=3.0cm]{figures/c5-10gpa-hf.pdf}
\label{hf_b5}
\end{subfigure}
\begin{subfigure}{0.17\textwidth}
\includegraphics[width=3.0cm,height=3.0cm]{figures/c5-10gpa-jcsf.pdf}
\label{vmc_b5}
\end{subfigure}
\begin{subfigure}{0.17\textwidth}
\includegraphics[width=3.0cm,height=3.0cm]{figures/c5-10gpa-tddft.pdf}
\label{pbe0_b5}
\end{subfigure}
\begin{subfigure}{0.17\textwidth}
\includegraphics[width=3.0cm,height=3.0cm]{figures/c5-10gpa-bse.pdf}
\label{bse_b5}
\end{subfigure}
\begin{subfigure}{0.17\textwidth}
\includegraphics[width=3.0cm,height=3.0cm]{figures/c5-10gpa-cis.pdf}
\label{cis_b5}
\end{subfigure}
\begin{subfigure}{0.17\textwidth}
%\includegraphics[width=3.0cm,height=3.0cm]{figures/c5-10gpa-jcis.pdf}
\begin{tikzpicture}
\node at (0,0){\includegraphics[width=3.0cm,height=3.0cm]{figures/c5-10gpa-jcis.pdf}};
\draw[] node at (2,0){\bf b5};
\end{tikzpicture}
\label{dmc_b5}
\end{subfigure}

\caption{Excitation-induced density difference, $\Delta\rho({\bf r})$, for
nuclear configurations {\bf b1}--{\bf b5} at $\rho/\rho_0=4.47$.
}
\label{fig:drho-b1-b5}
\end{figure*}

% 10gpa 6-10 %%%%%%%%%%%%%%%%%%%%%%%%%%%%%%%%%%%%%%%%%%%%%%%%%%%%%%%%%%%%%%%%%%%%%%%%%%%%%%%%%%

\begin{figure*}[h]

\hspace{-1.0cm}
\begin{subfigure}{0.17\textwidth}
\captionsetup{labelformat=empty}
\caption{{\em 1CSF0}}
\includegraphics[width=3.0cm,height=3.0cm]{figures/c6-10gpa-hf.pdf}
\label{hf_b6}
\end{subfigure}
\begin{subfigure}{0.17\textwidth}
\captionsetup{labelformat=empty}
\caption{DMC {\em J1CSF}}
\includegraphics[width=3.0cm,height=3.0cm]{figures/c6-10gpa-jcsf.pdf}
\label{vmc_b6}
\end{subfigure}
\begin{subfigure}{0.17\textwidth}
\captionsetup{labelformat=empty}
\caption{TDDFT}
\includegraphics[width=3.0cm,height=3.0cm]{figures/c6-10gpa-tddft.pdf}
\label{pbe0_b6}
\end{subfigure}
\begin{subfigure}{0.17\textwidth}
\captionsetup{labelformat=empty}
\caption{BSE}
\includegraphics[width=3.0cm,height=3.0cm]{figures/c6-10gpa-bse.pdf}
\label{bse_b6}
\end{subfigure}
\begin{subfigure}{0.17\textwidth}
\captionsetup{labelformat=empty}
\caption{{\em CIS0}}
\includegraphics[width=3.0cm,height=3.0cm]{figures/c6-10gpa-cis.pdf}
\label{cis_b6}
\end{subfigure}
\begin{subfigure}{0.17\textwidth}
\captionsetup{labelformat=empty}
\caption{DMC {\em JCIS}}
%\includegraphics[width=3.0cm,height=3.0cm]{figures/c6-10gpa-jcis.pdf}
\begin{tikzpicture}
\node at (0,0){\includegraphics[width=3.0cm,height=3.0cm]{figures/c6-10gpa-jcis.pdf}};
\draw[] node at (2,0){\bf b6};
\end{tikzpicture}
\label{dmc_b6}
\end{subfigure}

\hspace{-1.0cm}
\begin{subfigure}{0.17\textwidth}
\includegraphics[width=3.0cm,height=3.0cm]{figures/c7-10gpa-hf.pdf}
\label{hf_b7}
\end{subfigure}
\begin{subfigure}{0.17\textwidth}
\includegraphics[width=3.0cm,height=3.0cm]{figures/c7-10gpa-jcsf.pdf}
\label{vmc_b7}
\end{subfigure}
\begin{subfigure}{0.17\textwidth}
\includegraphics[width=3.0cm,height=3.0cm]{figures/c7-10gpa-tddft.pdf}
\label{pbe0_b7}
\end{subfigure}
\begin{subfigure}{0.17\textwidth}
\includegraphics[width=3.0cm,height=3.0cm]{figures/c7-10gpa-bse.pdf}
\label{bse_b7}
\end{subfigure}
\begin{subfigure}{0.17\textwidth}
\includegraphics[width=3.0cm,height=3.0cm]{figures/c7-10gpa-cis.pdf}
\label{cis_b7}
\end{subfigure}
\begin{subfigure}{0.17\textwidth}
%\includegraphics[width=3.0cm,height=3.0cm]{figures/c7-10gpa-jcis.pdf}
\begin{tikzpicture}
\node at (0,0){\includegraphics[width=3.0cm,height=3.0cm]{figures/c7-10gpa-jcis.pdf}};
\draw[] node at (2,0){\bf b7};
\end{tikzpicture}
\label{dmc_b7}
\end{subfigure}

\hspace{-1.0cm}
\begin{subfigure}{0.17\textwidth}
\includegraphics[width=3.0cm,height=3.0cm]{figures/c8-10gpa-hf.pdf}
\label{hf_b8}
\end{subfigure}
\begin{subfigure}{0.17\textwidth}
\includegraphics[width=3.0cm,height=3.0cm]{figures/c8-10gpa-jcsf.pdf}
\label{vmc_b8}
\end{subfigure}
\begin{subfigure}{0.17\textwidth}
\includegraphics[width=3.0cm,height=3.0cm]{figures/c8-10gpa-tddft.pdf}
\label{pbe0_b8}
\end{subfigure}
\begin{subfigure}{0.17\textwidth}
\includegraphics[width=3.0cm,height=3.0cm]{figures/c8-10gpa-bse.pdf}
\label{bse_b8}
\end{subfigure}
\begin{subfigure}{0.17\textwidth}
\includegraphics[width=3.0cm,height=3.0cm]{figures/c8-10gpa-cis.pdf}
\label{cis_b8}
\end{subfigure}
\begin{subfigure}{0.17\textwidth}
%\includegraphics[width=3.0cm,height=3.0cm]{figures/c8-10gpa-jcis.pdf}
\begin{tikzpicture}
\node at (0,0){\includegraphics[width=3.0cm,height=3.0cm]{figures/c8-10gpa-jcis.pdf}};
\draw[] node at (2,0){\bf b8};
\end{tikzpicture}
\label{dmc_b8}
\end{subfigure}

\hspace{-1.0cm}
\begin{subfigure}{0.17\textwidth}
\includegraphics[width=3.0cm,height=3.0cm]{figures/c9-10gpa-hf.pdf}
\label{hf_b9}
\end{subfigure}
\begin{subfigure}{0.17\textwidth}
\includegraphics[width=3.0cm,height=3.0cm]{figures/c9-10gpa-jcsf.pdf}
\label{vmc_b9}
\end{subfigure}
\begin{subfigure}{0.17\textwidth}
\includegraphics[width=3.0cm,height=3.0cm]{figures/c9-10gpa-tddft.pdf}
\label{pbe0_b9}
\end{subfigure}
\begin{subfigure}{0.17\textwidth}
\includegraphics[width=3.0cm,height=3.0cm]{figures/c9-10gpa-bse.pdf}
\label{bse_b9}
\end{subfigure}
\begin{subfigure}{0.17\textwidth}
\includegraphics[width=3.0cm,height=3.0cm]{figures/c9-10gpa-cis.pdf}
\label{cis_b9}
\end{subfigure}
\begin{subfigure}{0.17\textwidth}
%\includegraphics[width=3.0cm,height=3.0cm]{figures/c9-10gpa-jcis.pdf}
\begin{tikzpicture}
\node at (0,0){\includegraphics[width=3.0cm,height=3.0cm]{figures/c9-10gpa-jcis.pdf}};
\draw[] node at (2,0){\bf b9};
\end{tikzpicture}
\label{dmc_b9}
\end{subfigure}

\hspace{-1.0cm}
\begin{subfigure}{0.17\textwidth}
\includegraphics[width=3.0cm,height=3.0cm]{figures/c10-10gpa-hf.pdf}
\label{hf_b10}
\end{subfigure}
\begin{subfigure}{0.17\textwidth}
\includegraphics[width=3.0cm,height=3.0cm]{figures/c10-10gpa-jcsf.pdf}
\label{vmc_b10}
\end{subfigure}
\begin{subfigure}{0.17\textwidth}
\includegraphics[width=3.0cm,height=3.0cm]{figures/c10-10gpa-tddft.pdf}
\label{pbe0_b10}
\end{subfigure}
\begin{subfigure}{0.17\textwidth}
\includegraphics[width=3.0cm,height=3.0cm]{figures/c10-10gpa-bse.pdf}
\label{bse_b10}
\end{subfigure}
\begin{subfigure}{0.17\textwidth}
\includegraphics[width=3.0cm,height=3.0cm]{figures/c10-10gpa-cis.pdf}
\label{cis_b10}
\end{subfigure}
\begin{subfigure}{0.17\textwidth}
%\includegraphics[width=3.0cm,height=3.0cm]{figures/c10-10gpa-jcis.pdf}
\begin{tikzpicture}
\node at (0,0){\includegraphics[width=3.0cm,height=3.0cm]{figures/c10-10gpa-jcis.pdf}};
\draw[] node at (2,0){\bf b10};
\end{tikzpicture}
\label{dmc_b10}
\end{subfigure}

\caption{Excitation-induced density difference, $\Delta\rho({\bf r})$, for
nuclear configurations {\bf b6}--{\bf b10} at $\rho/\rho_0=4.47$.
}
\label{fig:drho-b6-b10}
\end{figure*}


% 10gpa 11-15 %%%%%%%%%%%%%%%%%%%%%%%%%%%%%%%%%%%%%%%%%%%%%%%%%%%%%%%%%%%%%%%%%%%%%%%%%%%%%%%%%%%

\begin{figure*}[h]

\hspace{-1.0cm}
\begin{subfigure}{0.17\textwidth}
\captionsetup{labelformat=empty}
\caption{{\em 1CSF0}}
\includegraphics[width=3.0cm,height=3.0cm]{figures/c11-10gpa-hf.pdf}
\label{hf_b11}
\end{subfigure}
\begin{subfigure}{0.17\textwidth}
\captionsetup{labelformat=empty}
\caption{DMC {\em J1CSF}}
\includegraphics[width=3.0cm,height=3.0cm]{figures/c11-10gpa-jcsf.pdf}
\label{vmc_b11}
\end{subfigure}
\begin{subfigure}{0.17\textwidth}
\captionsetup{labelformat=empty}
\caption{TDDFT}
\includegraphics[width=3.0cm,height=3.0cm]{figures/c11-10gpa-tddft.pdf}
\label{pbe0_b11}
\end{subfigure}
\begin{subfigure}{0.17\textwidth}
\captionsetup{labelformat=empty}
\caption{BSE}
\includegraphics[width=3.0cm,height=3.0cm]{figures/c11-10gpa-bse.pdf}
\label{bse_b11}
\end{subfigure}
\begin{subfigure}{0.17\textwidth}
\captionsetup{labelformat=empty}
\caption{{\em CIS0}}
\includegraphics[width=3.0cm,height=3.0cm]{figures/c11-10gpa-cis.pdf}
\label{cis_b11}
\end{subfigure}
\begin{subfigure}{0.17\textwidth}
\captionsetup{labelformat=empty}
\caption{DMC {\em JCIS}}
%\includegraphics[width=3.0cm,height=3.0cm]{figures/c11-10gpa-jcis.pdf}
\begin{tikzpicture}
\node at (0,0){\includegraphics[width=3.0cm,height=3.0cm]{figures/c11-10gpa-jcis.pdf}};
\draw[] node at (2,0){\bf b11};
\end{tikzpicture}
\label{dmc_b11}
\end{subfigure}

\hspace{-1.0cm}
\begin{subfigure}{0.17\textwidth}
\includegraphics[width=3.0cm,height=3.0cm]{figures/c12-10gpa-hf.pdf}
\label{hf_b12}
\end{subfigure}
\begin{subfigure}{0.17\textwidth}
\includegraphics[width=3.0cm,height=3.0cm]{figures/c12-10gpa-jcsf.pdf}
\label{vmc_b12}
\end{subfigure}
\begin{subfigure}{0.17\textwidth}
\includegraphics[width=3.0cm,height=3.0cm]{figures/c12-10gpa-tddft.pdf}
\label{pbe0_b12}
\end{subfigure}
\begin{subfigure}{0.17\textwidth}
\includegraphics[width=3.0cm,height=3.0cm]{figures/c12-10gpa-bse.pdf}
\label{bse_b12}
\end{subfigure}
\begin{subfigure}{0.17\textwidth}
\includegraphics[width=3.0cm,height=3.0cm]{figures/c12-10gpa-cis.pdf}
\label{cis_b12}
\end{subfigure}
\begin{subfigure}{0.17\textwidth}
%\includegraphics[width=3.0cm,height=3.0cm]{figures/c12-10gpa-jcis.pdf}
\begin{tikzpicture}
\node at (0,0){\includegraphics[width=3.0cm,height=3.0cm]{figures/c12-10gpa-jcis.pdf}};
\draw[] node at (2,0){\bf b12};
\end{tikzpicture}
\label{dmc_b12}
\end{subfigure}

\hspace{-1.0cm}
\begin{subfigure}{0.17\textwidth}
\includegraphics[width=3.0cm,height=3.0cm]{figures/c13-10gpa-hf.pdf}
\label{hf_b13}
\end{subfigure}
\begin{subfigure}{0.17\textwidth}
\includegraphics[width=3.0cm,height=3.0cm]{figures/c13-10gpa-jcsf.pdf}
\label{vmc_b13}
\end{subfigure}
\begin{subfigure}{0.17\textwidth}
\includegraphics[width=3.0cm,height=3.0cm]{figures/c13-10gpa-tddft.pdf}
\label{pbe0_b13}
\end{subfigure}
\begin{subfigure}{0.17\textwidth}
\includegraphics[width=3.0cm,height=3.0cm]{figures/c13-10gpa-bse.pdf}
\label{bse_b13}
\end{subfigure}
\begin{subfigure}{0.17\textwidth}
\includegraphics[width=3.0cm,height=3.0cm]{figures/c13-10gpa-cis.pdf}
\label{cis_b13}
\end{subfigure}
\begin{subfigure}{0.17\textwidth}
%\includegraphics[width=3.0cm,height=3.0cm]{figures/c13-10gpa-jcis.pdf}
\begin{tikzpicture}
\node at (0,0){\includegraphics[width=3.0cm,height=3.0cm]{figures/c13-10gpa-jcis.pdf}};
\draw[] node at (2,0){\bf b13};
\end{tikzpicture}
\label{dmc_b13}
\end{subfigure}

\hspace{-1.0cm}
\begin{subfigure}{0.17\textwidth}
\includegraphics[width=3.0cm,height=3.0cm]{figures/c14-10gpa-hf.pdf}
\label{hf_b14}
\end{subfigure}
\begin{subfigure}{0.17\textwidth}
\includegraphics[width=3.0cm,height=3.0cm]{figures/c14-10gpa-jcsf.pdf}
\label{vmc_b14}
\end{subfigure}
\begin{subfigure}{0.17\textwidth}
\includegraphics[width=3.0cm,height=3.0cm]{figures/c14-10gpa-tddft.pdf}
\label{pbe0_b14}
\end{subfigure}
\begin{subfigure}{0.17\textwidth}
\includegraphics[width=3.0cm,height=3.0cm]{figures/c14-10gpa-bse.pdf}
\label{bse_b14}
\end{subfigure}
\begin{subfigure}{0.17\textwidth}
\includegraphics[width=3.0cm,height=3.0cm]{figures/c14-10gpa-cis.pdf}
\label{cis_b14}
\end{subfigure}
\begin{subfigure}{0.17\textwidth}
%\includegraphics[width=3.0cm,height=3.0cm]{figures/c14-10gpa-jcis.pdf}
\begin{tikzpicture}
\node at (0,0){\includegraphics[width=3.0cm,height=3.0cm]{figures/c14-10gpa-jcis.pdf}};
\draw[] node at (2,0){\bf b14};
\end{tikzpicture}
\label{dmc_b14}
\end{subfigure}

\hspace{-1.0cm}
\begin{subfigure}{0.17\textwidth}
\includegraphics[width=3.0cm,height=3.0cm]{figures/c15-10gpa-hf.pdf}
\label{hf_b15}
\end{subfigure}
\begin{subfigure}{0.17\textwidth}
\includegraphics[width=3.0cm,height=3.0cm]{figures/c15-10gpa-jcsf.pdf}
\label{vmc_b15}
\end{subfigure}
\begin{subfigure}{0.17\textwidth}
\includegraphics[width=3.0cm,height=3.0cm]{figures/c15-10gpa-tddft.pdf}
\label{pbe0_b15}
\end{subfigure}
\begin{subfigure}{0.17\textwidth}
\includegraphics[width=3.0cm,height=3.0cm]{figures/c15-10gpa-bse.pdf}
\label{bse_b15}
\end{subfigure}
\begin{subfigure}{0.17\textwidth}
\includegraphics[width=3.0cm,height=3.0cm]{figures/c15-10gpa-cis.pdf}
\label{cis_b15}
\end{subfigure}
\begin{subfigure}{0.17\textwidth}
%\includegraphics[width=3.0cm,height=3.0cm]{figures/c15-10gpa-jcis.pdf}
\begin{tikzpicture}
\node at (0,0){\includegraphics[width=3.0cm,height=3.0cm]{figures/c15-10gpa-jcis.pdf}};
\draw[] node at (2,0){\bf b15};
\end{tikzpicture}
\label{dmc_b15}
\end{subfigure}

\caption{Excitation-induced density difference, $\Delta\rho({\bf r})$, for
nuclear configurations {\bf b11}--{\bf b15} at $\rho/\rho_0=4.47$.
}
\label{fig:drho-b11-b15}
\end{figure*}

% 10gpa 16-20 %%%%%%%%%%%%%%%%%%%%%%%%%%%%%%%%%%%%%%%%%%%%%%%%%%%%%%%%%%%%%%%%%%%%%%%%%%%%%%%%%%

\begin{figure*}[h]

\hspace{-1.0cm}
\begin{subfigure}{0.17\textwidth}
\captionsetup{labelformat=empty}
\caption{{\em 1CSF0}}
\includegraphics[width=3.0cm,height=3.0cm]{figures/c16-10gpa-hf.pdf}
\label{hf_b16}
\end{subfigure}
\begin{subfigure}{0.17\textwidth}
\captionsetup{labelformat=empty}
\caption{DMC {\em J1CSF}}
\includegraphics[width=3.0cm,height=3.0cm]{figures/c16-10gpa-jcsf.pdf}
\label{vmc_b16}
\end{subfigure}
\begin{subfigure}{0.17\textwidth}
\captionsetup{labelformat=empty}
\caption{TDDFT}
\includegraphics[width=3.0cm,height=3.0cm]{figures/c16-10gpa-tddft.pdf}
\label{pbe0_b16}
\end{subfigure}
\begin{subfigure}{0.17\textwidth}
\captionsetup{labelformat=empty}
\caption{BSE}
\includegraphics[width=3.0cm,height=3.0cm]{figures/c16-10gpa-bse.pdf}
\label{bse_b16}
\end{subfigure}
\begin{subfigure}{0.17\textwidth}
\captionsetup{labelformat=empty}
\caption{{\em CIS0}}
\includegraphics[width=3.0cm,height=3.0cm]{figures/c16-10gpa-cis.pdf}
\label{cis_b16}
\end{subfigure}
\begin{subfigure}{0.17\textwidth}
\captionsetup{labelformat=empty}
\caption{DMC {\em JCIS}}
%\includegraphics[width=3.0cm,height=3.0cm]{figures/c16-10gpa-jcis.pdf}
\begin{tikzpicture}
\node at (0,0){\includegraphics[width=3.0cm,height=3.0cm]{figures/c16-10gpa-jcis.pdf}};
\draw[] node at (2,0){\bf b16};
\end{tikzpicture}
\label{dmc_b16}
\end{subfigure}

\hspace{-1.0cm}
\begin{subfigure}{0.17\textwidth}
\includegraphics[width=3.0cm,height=3.0cm]{figures/c17-10gpa-hf.pdf}
\label{hf_b17}
\end{subfigure}
\begin{subfigure}{0.17\textwidth}
\includegraphics[width=3.0cm,height=3.0cm]{figures/c17-10gpa-jcsf.pdf}
\label{vmc_b17}
\end{subfigure}
\begin{subfigure}{0.17\textwidth}
\includegraphics[width=3.0cm,height=3.0cm]{figures/c17-10gpa-tddft.pdf}
\label{pbe0_b17}
\end{subfigure}
\begin{subfigure}{0.17\textwidth}
\includegraphics[width=3.0cm,height=3.0cm]{figures/c17-10gpa-bse.pdf}
\label{bse_b17}
\end{subfigure}
\begin{subfigure}{0.17\textwidth}
\includegraphics[width=3.0cm,height=3.0cm]{figures/c17-10gpa-cis.pdf}
\label{cis_b17}
\end{subfigure}
\begin{subfigure}{0.17\textwidth}
%\includegraphics[width=3.0cm,height=3.0cm]{figures/c17-10gpa-jcis.pdf}
\begin{tikzpicture}
\node at (0,0){\includegraphics[width=3.0cm,height=3.0cm]{figures/c17-10gpa-jcis.pdf}};
\draw[] node at (2,0){\bf b17};
\end{tikzpicture}
\label{dmc_b17}
\end{subfigure}

\hspace{-1.0cm}
\begin{subfigure}{0.17\textwidth}
\includegraphics[width=3.0cm,height=3.0cm]{figures/c18-10gpa-hf.pdf}
\label{hf_b18}
\end{subfigure}
\begin{subfigure}{0.17\textwidth}
\includegraphics[width=3.0cm,height=3.0cm]{figures/c18-10gpa-jcsf.pdf}
\label{vmc_b18}
\end{subfigure}
\begin{subfigure}{0.17\textwidth}
\includegraphics[width=3.0cm,height=3.0cm]{figures/c18-10gpa-tddft.pdf}
\label{pbe0_b18}
\end{subfigure}
\begin{subfigure}{0.17\textwidth}
\includegraphics[width=3.0cm,height=3.0cm]{figures/c18-10gpa-bse.pdf}
\label{bse_b18}
\end{subfigure}
\begin{subfigure}{0.17\textwidth}
\includegraphics[width=3.0cm,height=3.0cm]{figures/c18-10gpa-cis.pdf}
\label{cis_b18}
\end{subfigure}
\begin{subfigure}{0.17\textwidth}
%\includegraphics[width=3.0cm,height=3.0cm]{figures/c18-10gpa-jcis.pdf}
\begin{tikzpicture}
\node at (0,0){\includegraphics[width=3.0cm,height=3.0cm]{figures/c18-10gpa-jcis.pdf}};
\draw[] node at (2,0){\bf b18};
\end{tikzpicture}
\label{dmc_b18}
\end{subfigure}

\hspace{-1.0cm}
\begin{subfigure}{0.17\textwidth}
\includegraphics[width=3.0cm,height=3.0cm]{figures/c19-10gpa-hf.pdf}
\label{hf_b19}
\end{subfigure}
\begin{subfigure}{0.17\textwidth}
\includegraphics[width=3.0cm,height=3.0cm]{figures/c19-10gpa-jcsf.pdf}
\label{vmc_b19}
\end{subfigure}
\begin{subfigure}{0.17\textwidth}
\includegraphics[width=3.0cm,height=3.0cm]{figures/c19-10gpa-tddft.pdf}
\label{pbe0_b19}
\end{subfigure}
\begin{subfigure}{0.17\textwidth}
\includegraphics[width=3.0cm,height=3.0cm]{figures/c19-10gpa-bse.pdf}
\label{bse_b19}
\end{subfigure}
\begin{subfigure}{0.17\textwidth}
\includegraphics[width=3.0cm,height=3.0cm]{figures/c19-10gpa-cis.pdf}
\label{cis_b19}
\end{subfigure}
\begin{subfigure}{0.17\textwidth}
%\includegraphics[width=3.0cm,height=3.0cm]{figures/c19-10gpa-jcis.pdf}
\begin{tikzpicture}
\node at (0,0){\includegraphics[width=3.0cm,height=3.0cm]{figures/c19-10gpa-jcis.pdf}};
\draw[] node at (2,0){\bf b19};
\end{tikzpicture}
\label{dmc_b19}
\end{subfigure}

\hspace{-1.0cm}
\begin{subfigure}{0.17\textwidth}
\includegraphics[width=3.0cm,height=3.0cm]{figures/c20-10gpa-hf.pdf}
\label{hf_b20}
\end{subfigure}
\begin{subfigure}{0.17\textwidth}
\includegraphics[width=3.0cm,height=3.0cm]{figures/c20-10gpa-jcsf.pdf}
\label{vmc_b20}
\end{subfigure}
\begin{subfigure}{0.17\textwidth}
\includegraphics[width=3.0cm,height=3.0cm]{figures/c20-10gpa-tddft.pdf}
\label{pbe0_b20}
\end{subfigure}
\begin{subfigure}{0.17\textwidth}
\includegraphics[width=3.0cm,height=3.0cm]{figures/c20-10gpa-bse.pdf}
\label{bse_b20}
\end{subfigure}
\begin{subfigure}{0.17\textwidth}
\includegraphics[width=3.0cm,height=3.0cm]{figures/c20-10gpa-cis.pdf}
\label{cis_b20}
\end{subfigure}
\begin{subfigure}{0.17\textwidth}
%\includegraphics[width=3.0cm,height=3.0cm]{figures/c20-10gpa-jcis.pdf}
\begin{tikzpicture}
\node at (0,0){\includegraphics[width=3.0cm,height=3.0cm]{figures/c20-10gpa-jcis.pdf}};
\draw[] node at (2,0){\bf b20};
\end{tikzpicture}
\label{dmc_b20}
\end{subfigure}

\caption{Excitation-induced density difference, $\Delta\rho({\bf r})$, for
nuclear configurations {\bf b16}--{\bf b20} at $\rho/\rho_0=4.47$.
}
\label{fig:drho-b16-b20}
\end{figure*}



% 90gpa 1-5 %%%%%%%%%%%%%%%%%%%%%%%%%%%%%%%%%%%%%%%%%%%%%%%%%%%%%%%%%%%%%%%%%%%%%%%%%%%%%%%%%%%

\begin{figure*}[h]

\hspace{-1.0cm}
\begin{subfigure}{0.17\textwidth}
\captionsetup{labelformat=empty}
\caption{{\em 1CSF0}}
\includegraphics[width=3.0cm,height=3.0cm]{figures/c1-90gpa-hf.pdf}
\label{hf_c1}
\end{subfigure}
\begin{subfigure}{0.17\textwidth}
\captionsetup{labelformat=empty}
\caption{DMC {\em J1CSF}}
\includegraphics[width=3.0cm,height=3.0cm]{figures/c1-90gpa-jcsf.pdf}
\label{vmc_c1}
\end{subfigure}
\begin{subfigure}{0.17\textwidth}
\captionsetup{labelformat=empty}
\caption{TDDFT}
\includegraphics[width=3.0cm,height=3.0cm]{figures/c1-90gpa-tddft.pdf}
\label{pbe0_c1}
\end{subfigure}
\begin{subfigure}{0.17\textwidth}
\captionsetup{labelformat=empty}
\caption{BSE}
\includegraphics[width=3.0cm,height=3.0cm]{figures/c1-90gpa-bse.pdf}
\label{bse_c1}
\end{subfigure}
\begin{subfigure}{0.17\textwidth}
\captionsetup{labelformat=empty}
\caption{{\em CIS0}}
\includegraphics[width=3.0cm,height=3.0cm]{figures/c1-90gpa-cis.pdf}
\label{cis_c1}
\end{subfigure}
\begin{subfigure}{0.17\textwidth}
\captionsetup{labelformat=empty}
\caption{DMC {\em JCIS}}
%\includegraphics[width=3.0cm,height=3.0cm]{figures/c1-90gpa-jcis.pdf}
\begin{tikzpicture}
\node at (0,0){\includegraphics[width=3.0cm,height=3.0cm]{figures/c1-90gpa-jcis.pdf}};
\draw[] node at (2,0){\bf c1};
\end{tikzpicture}
\label{dmc_c1}
\end{subfigure}

\hspace{-1.0cm}
\begin{subfigure}{0.17\textwidth}
\includegraphics[width=3.0cm,height=3.0cm]{figures/c2-90gpa-hf.pdf}
\label{hf_c2}
\end{subfigure}
\begin{subfigure}{0.17\textwidth}
\includegraphics[width=3.0cm,height=3.0cm]{figures/c2-90gpa-jcsf.pdf}
\label{vmc_c2}
\end{subfigure}
\begin{subfigure}{0.17\textwidth}
\includegraphics[width=3.0cm,height=3.0cm]{figures/c2-90gpa-tddft.pdf}
\label{pbe0_c2}
\end{subfigure}
\begin{subfigure}{0.17\textwidth}
\includegraphics[width=3.0cm,height=3.0cm]{figures/c2-90gpa-bse.pdf}
\label{bse_c2}
\end{subfigure}
\begin{subfigure}{0.17\textwidth}
\includegraphics[width=3.0cm,height=3.0cm]{figures/c2-90gpa-cis.pdf}
\label{cis_c2}
\end{subfigure}
\begin{subfigure}{0.17\textwidth}
%\includegraphics[width=3.0cm,height=3.0cm]{figures/c2-90gpa-jcis.pdf}
\begin{tikzpicture}
\node at (0,0){\includegraphics[width=3.0cm,height=3.0cm]{figures/c2-90gpa-jcis.pdf}};
\draw[] node at (2,0){\bf c2};
\end{tikzpicture}
\label{dmc_c2}
\end{subfigure}

\hspace{-1.0cm}
\begin{subfigure}{0.17\textwidth}
\includegraphics[width=3.0cm,height=3.0cm]{figures/c3-90gpa-hf.pdf}
\label{hf_c3}
\end{subfigure}
\begin{subfigure}{0.17\textwidth}
\includegraphics[width=3.0cm,height=3.0cm]{figures/c3-90gpa-jcsf.pdf}
\label{vmc_c3}
\end{subfigure}
\begin{subfigure}{0.17\textwidth}
\includegraphics[width=3.0cm,height=3.0cm]{figures/c3-90gpa-tddft.pdf}
\label{pbe0_c3}
\end{subfigure}
\begin{subfigure}{0.17\textwidth}
\includegraphics[width=3.0cm,height=3.0cm]{figures/c3-90gpa-bse.pdf}
\label{bse_c3}
\end{subfigure}
\begin{subfigure}{0.17\textwidth}
\includegraphics[width=3.0cm,height=3.0cm]{figures/c3-90gpa-cis.pdf}
\label{cis_c3}
\end{subfigure}
\begin{subfigure}{0.17\textwidth}
%\includegraphics[width=3.0cm,height=3.0cm]{figures/c3-90gpa-jcis.pdf}
\begin{tikzpicture}
\node at (0,0){\includegraphics[width=3.0cm,height=3.0cm]{figures/c3-90gpa-jcis.pdf}};
\draw[] node at (2,0){\bf c3};
\end{tikzpicture}
\label{dmc_c3}
\end{subfigure}

\hspace{-1.0cm}
\begin{subfigure}{0.17\textwidth}
\includegraphics[width=3.0cm,height=3.0cm]{figures/c4-90gpa-hf.pdf}
\label{hf_c4}
\end{subfigure}
\begin{subfigure}{0.17\textwidth}
\includegraphics[width=3.0cm,height=3.0cm]{figures/c4-90gpa-jcsf.pdf}
\label{vmc_c4}
\end{subfigure}
\begin{subfigure}{0.17\textwidth}
\includegraphics[width=3.0cm,height=3.0cm]{figures/c4-90gpa-tddft.pdf}
\label{pbe0_c4}
\end{subfigure}
\begin{subfigure}{0.17\textwidth}
\includegraphics[width=3.0cm,height=3.0cm]{figures/c4-90gpa-bse.pdf}
\label{bse_c4}
\end{subfigure}
\begin{subfigure}{0.17\textwidth}
\includegraphics[width=3.0cm,height=3.0cm]{figures/c4-90gpa-cis.pdf}
\label{cis_c4}
\end{subfigure}
\begin{subfigure}{0.17\textwidth}
%\includegraphics[width=3.0cm,height=3.0cm]{figures/c4-90gpa-jcis.pdf}
\begin{tikzpicture}
\node at (0,0){\includegraphics[width=3.0cm,height=3.0cm]{figures/c4-90gpa-jcis.pdf}};
\draw[] node at (2,0){\bf c4};
\end{tikzpicture}
\label{dmc_c4}
\end{subfigure}

\hspace{-1.0cm}
\begin{subfigure}{0.17\textwidth}
\includegraphics[width=3.0cm,height=3.0cm]{figures/c5-90gpa-hf.pdf}
\label{hf_c5}
\end{subfigure}
\begin{subfigure}{0.17\textwidth}
\includegraphics[width=3.0cm,height=3.0cm]{figures/c5-90gpa-jcsf.pdf}
\label{vmc_c5}
\end{subfigure}
\begin{subfigure}{0.17\textwidth}
\includegraphics[width=3.0cm,height=3.0cm]{figures/c5-90gpa-tddft.pdf}
\label{pbe0_c5}
\end{subfigure}
\begin{subfigure}{0.17\textwidth}
\includegraphics[width=3.0cm,height=3.0cm]{figures/c5-90gpa-bse.pdf}
\label{bse_c5}
\end{subfigure}
\begin{subfigure}{0.17\textwidth}
\includegraphics[width=3.0cm,height=3.0cm]{figures/c5-90gpa-cis.pdf}
\label{cis_c5}
\end{subfigure}
\begin{subfigure}{0.17\textwidth}
%\includegraphics[width=3.0cm,height=3.0cm]{figures/c5-90gpa-jcis.pdf}
\begin{tikzpicture}
\node at (0,0){\includegraphics[width=3.0cm,height=3.0cm]{figures/c5-90gpa-jcis.pdf}};
\draw[] node at (2,0){\bf c5};
\end{tikzpicture}
\label{dmc_c5}
\end{subfigure}

\caption{Excitation-induced density difference, $\Delta\rho({\bf r})$, for
nuclear configurations {\bf c1}--{\bf c5} at $\rho/\rho_0=8.48$.
}
\label{fig:drho-c1-c5}
\end{figure*}

% 90gpa 6-10 %%%%%%%%%%%%%%%%%%%%%%%%%%%%%%%%%%%%%%%%%%%%%%%%%%%%%%%%%%%%%%%%%%%%%%%%%%%%%%%%%%

\begin{figure*}[h]

\hspace{-1.0cm}
\begin{subfigure}{0.17\textwidth}
\captionsetup{labelformat=empty}
\caption{{\em 1CSF0}}
\includegraphics[width=3.0cm,height=3.0cm]{figures/c6-90gpa-hf.pdf}
\label{hf_c6}
\end{subfigure}
\begin{subfigure}{0.17\textwidth}
\captionsetup{labelformat=empty}
\caption{DMC {\em J1CSF}}
\includegraphics[width=3.0cm,height=3.0cm]{figures/c6-90gpa-jcsf.pdf}
\label{vmc_c6}
\end{subfigure}
\begin{subfigure}{0.17\textwidth}
\captionsetup{labelformat=empty}
\caption{TDDFT}
\includegraphics[width=3.0cm,height=3.0cm]{figures/c6-90gpa-tddft.pdf}
\label{pbe0_c6}
\end{subfigure}
\begin{subfigure}{0.17\textwidth}
\captionsetup{labelformat=empty}
\caption{BSE}
\includegraphics[width=3.0cm,height=3.0cm]{figures/c6-90gpa-bse.pdf}
\label{bse_c6}
\end{subfigure}
\begin{subfigure}{0.17\textwidth}
\captionsetup{labelformat=empty}
\caption{{\em CIS0}}
\includegraphics[width=3.0cm,height=3.0cm]{figures/c6-90gpa-cis.pdf}
\label{cis_c6}
\end{subfigure}
\begin{subfigure}{0.17\textwidth}
\captionsetup{labelformat=empty}
\caption{DMC {\em JCIS}}
%\includegraphics[width=3.0cm,height=3.0cm]{figures/c6-90gpa-jcis.pdf}
\begin{tikzpicture}
\node at (0,0){\includegraphics[width=3.0cm,height=3.0cm]{figures/c6-90gpa-jcis.pdf}};
\draw[] node at (2,0){\bf c6};
\end{tikzpicture}
\label{dmc_c6}
\end{subfigure}

\hspace{-1.0cm}
\begin{subfigure}{0.17\textwidth}
\includegraphics[width=3.0cm,height=3.0cm]{figures/c7-90gpa-hf.pdf}
\label{hf_c7}
\end{subfigure}
\begin{subfigure}{0.17\textwidth}
\includegraphics[width=3.0cm,height=3.0cm]{figures/c7-90gpa-jcsf.pdf}
\label{vmc_c7}
\end{subfigure}
\begin{subfigure}{0.17\textwidth}
\includegraphics[width=3.0cm,height=3.0cm]{figures/c7-90gpa-tddft.pdf}
\label{pbe0_c7}
\end{subfigure}
\begin{subfigure}{0.17\textwidth}
\includegraphics[width=3.0cm,height=3.0cm]{figures/c7-90gpa-bse.pdf}
\label{bse_c7}
\end{subfigure}
\begin{subfigure}{0.17\textwidth}
\includegraphics[width=3.0cm,height=3.0cm]{figures/c7-90gpa-cis.pdf}
\label{cis_c7}
\end{subfigure}
\begin{subfigure}{0.17\textwidth}
%\includegraphics[width=3.0cm,height=3.0cm]{figures/c7-90gpa-jcis.pdf}
\begin{tikzpicture}
\node at (0,0){\includegraphics[width=3.0cm,height=3.0cm]{figures/c7-90gpa-jcis.pdf}};
\draw[] node at (2,0){\bf c7};
\end{tikzpicture}
\label{dmc_c7}
\end{subfigure}

\hspace{-1.0cm}
\begin{subfigure}{0.17\textwidth}
\includegraphics[width=3.0cm,height=3.0cm]{figures/c8-90gpa-hf.pdf}
\label{hf_c8}
\end{subfigure}
\begin{subfigure}{0.17\textwidth}
\includegraphics[width=3.0cm,height=3.0cm]{figures/c8-90gpa-jcsf.pdf}
\label{vmc_c8}
\end{subfigure}
\begin{subfigure}{0.17\textwidth}
\includegraphics[width=3.0cm,height=3.0cm]{figures/c8-90gpa-tddft.pdf}
\label{pbe0_c8}
\end{subfigure}
\begin{subfigure}{0.17\textwidth}
\includegraphics[width=3.0cm,height=3.0cm]{figures/c8-90gpa-bse.pdf}
\label{bse_c8}
\end{subfigure}
\begin{subfigure}{0.17\textwidth}
\includegraphics[width=3.0cm,height=3.0cm]{figures/c8-90gpa-cis.pdf}
\label{cis_c8}
\end{subfigure}
\begin{subfigure}{0.17\textwidth}
%\includegraphics[width=3.0cm,height=3.0cm]{figures/c8-90gpa-jcis.pdf}
\begin{tikzpicture}
\node at (0,0){\includegraphics[width=3.0cm,height=3.0cm]{figures/c8-90gpa-jcis.pdf}};
\draw[] node at (2,0){\bf c8};
\end{tikzpicture}
\label{dmc_c8}
\end{subfigure}

\hspace{-1.0cm}
\begin{subfigure}{0.17\textwidth}
\includegraphics[width=3.0cm,height=3.0cm]{figures/c9-90gpa-hf.pdf}
\label{hf_c9}
\end{subfigure}
\begin{subfigure}{0.17\textwidth}
\includegraphics[width=3.0cm,height=3.0cm]{figures/c9-90gpa-jcsf.pdf}
\label{vmc_c9}
\end{subfigure}
\begin{subfigure}{0.17\textwidth}
\includegraphics[width=3.0cm,height=3.0cm]{figures/c9-90gpa-tddft.pdf}
\label{pbe0_c9}
\end{subfigure}
\begin{subfigure}{0.17\textwidth}
\includegraphics[width=3.0cm,height=3.0cm]{figures/c9-90gpa-bse.pdf}
\label{bse_c9}
\end{subfigure}
\begin{subfigure}{0.17\textwidth}
\includegraphics[width=3.0cm,height=3.0cm]{figures/c9-90gpa-cis.pdf}
\label{cis_c9}
\end{subfigure}
\begin{subfigure}{0.17\textwidth}
%\includegraphics[width=3.0cm,height=3.0cm]{figures/c9-90gpa-jcis.pdf}
\begin{tikzpicture}
\node at (0,0){\includegraphics[width=3.0cm,height=3.0cm]{figures/c9-90gpa-jcis.pdf}};
\draw[] node at (2,0){\bf c9};
\end{tikzpicture}
\label{dmc_c9}
\end{subfigure}

\hspace{-1.0cm}
\begin{subfigure}{0.17\textwidth}
\includegraphics[width=3.0cm,height=3.0cm]{figures/c10-90gpa-hf.pdf}
\label{hf_c10}
\end{subfigure}
\begin{subfigure}{0.17\textwidth}
\includegraphics[width=3.0cm,height=3.0cm]{figures/c10-90gpa-jcsf.pdf}
\label{vmc_c10}
\end{subfigure}
\begin{subfigure}{0.17\textwidth}
\includegraphics[width=3.0cm,height=3.0cm]{figures/c10-90gpa-tddft.pdf}
\label{pbe0_c10}
\end{subfigure}
\begin{subfigure}{0.17\textwidth}
\includegraphics[width=3.0cm,height=3.0cm]{figures/c10-90gpa-bse.pdf}
\label{bse_c10}
\end{subfigure}
\begin{subfigure}{0.17\textwidth}
\includegraphics[width=3.0cm,height=3.0cm]{figures/c10-90gpa-cis.pdf}
\label{cis_c10}
\end{subfigure}
\begin{subfigure}{0.17\textwidth}
%\includegraphics[width=3.0cm,height=3.0cm]{figures/c10-90gpa-jcis.pdf}
\begin{tikzpicture}
\node at (0,0){\includegraphics[width=3.0cm,height=3.0cm]{figures/c10-90gpa-jcis.pdf}};
\draw[] node at (2,0){\bf c10};
\end{tikzpicture}
\label{dmc_c10}
\end{subfigure}

\caption{Excitation-induced density difference, $\Delta\rho({\bf r})$, for
nuclear configurations {\bf c6}--{\bf c10} at $\rho/\rho_0=8.48$.
}
\label{fig:drho-c6-c10}
\end{figure*}


% 90gpa 11-15 %%%%%%%%%%%%%%%%%%%%%%%%%%%%%%%%%%%%%%%%%%%%%%%%%%%%%%%%%%%%%%%%%%%%%%%%%%%%%%%%%%%

\begin{figure*}[h]

\hspace{-1.0cm}
\begin{subfigure}{0.17\textwidth}
\captionsetup{labelformat=empty}
\caption{{\em 1CSF0}}
\includegraphics[width=3.0cm,height=3.0cm]{figures/c11-90gpa-hf.pdf}
\label{hf_c11}
\end{subfigure}
\begin{subfigure}{0.17\textwidth}
\captionsetup{labelformat=empty}
\caption{DMC {\em J1CSF}}
\includegraphics[width=3.0cm,height=3.0cm]{figures/c11-90gpa-jcsf.pdf}
\label{vmc_c11}
\end{subfigure}
\begin{subfigure}{0.17\textwidth}
\captionsetup{labelformat=empty}
\caption{TDDFT}
\includegraphics[width=3.0cm,height=3.0cm]{figures/c11-90gpa-tddft.pdf}
\label{pbe0_c11}
\end{subfigure}
\begin{subfigure}{0.17\textwidth}
\captionsetup{labelformat=empty}
\caption{BSE}
\includegraphics[width=3.0cm,height=3.0cm]{figures/c11-90gpa-bse.pdf}
\label{bse_c11}
\end{subfigure}
\begin{subfigure}{0.17\textwidth}
\captionsetup{labelformat=empty}
\caption{{\em CIS0}}
\includegraphics[width=3.0cm,height=3.0cm]{figures/c11-90gpa-cis.pdf}
\label{cis_c11}
\end{subfigure}
\begin{subfigure}{0.17\textwidth}
\captionsetup{labelformat=empty}
\caption{DMC {\em JCIS}}
%\includegraphics[width=3.0cm,height=3.0cm]{figures/c11-90gpa-jcis.pdf}
\begin{tikzpicture}
\node at (0,0){\includegraphics[width=3.0cm,height=3.0cm]{figures/c11-90gpa-jcis.pdf}};
\draw[] node at (2,0){\bf c11};
\end{tikzpicture}
\label{dmc_c11}
\end{subfigure}

\hspace{-1.0cm}
\begin{subfigure}{0.17\textwidth}
\includegraphics[width=3.0cm,height=3.0cm]{figures/c12-90gpa-hf.pdf}
\label{hf_c12}
\end{subfigure}
\begin{subfigure}{0.17\textwidth}
\includegraphics[width=3.0cm,height=3.0cm]{figures/c12-90gpa-jcsf.pdf}
\label{vmc_c12}
\end{subfigure}
\begin{subfigure}{0.17\textwidth}
\includegraphics[width=3.0cm,height=3.0cm]{figures/c12-90gpa-tddft.pdf}
\label{pbe0_c12}
\end{subfigure}
\begin{subfigure}{0.17\textwidth}
\includegraphics[width=3.0cm,height=3.0cm]{figures/c12-90gpa-bse.pdf}
\label{bse_c12}
\end{subfigure}
\begin{subfigure}{0.17\textwidth}
\includegraphics[width=3.0cm,height=3.0cm]{figures/c12-90gpa-cis.pdf}
\label{cis_c12}
\end{subfigure}
\begin{subfigure}{0.17\textwidth}
%\includegraphics[width=3.0cm,height=3.0cm]{figures/c12-90gpa-jcis.pdf}
\begin{tikzpicture}
\node at (0,0){\includegraphics[width=3.0cm,height=3.0cm]{figures/c2-90gpa-jcis.pdf}};
\draw[] node at (2,0){\bf c12};
\end{tikzpicture}
\label{dmc_c12}
\end{subfigure}

\hspace{-1.0cm}
\begin{subfigure}{0.17\textwidth}
\includegraphics[width=3.0cm,height=3.0cm]{figures/c13-90gpa-hf.pdf}
\label{hf_c13}
\end{subfigure}
\begin{subfigure}{0.17\textwidth}
\includegraphics[width=3.0cm,height=3.0cm]{figures/c13-90gpa-jcsf.pdf}
\label{vmc_c13}
\end{subfigure}
\begin{subfigure}{0.17\textwidth}
\includegraphics[width=3.0cm,height=3.0cm]{figures/c13-90gpa-tddft.pdf}
\label{pbe0_c13}
\end{subfigure}
\begin{subfigure}{0.17\textwidth}
\includegraphics[width=3.0cm,height=3.0cm]{figures/c13-90gpa-bse.pdf}
\label{bse_c13}
\end{subfigure}
\begin{subfigure}{0.17\textwidth}
\includegraphics[width=3.0cm,height=3.0cm]{figures/c13-90gpa-cis.pdf}
\label{cis_c13}
\end{subfigure}
\begin{subfigure}{0.17\textwidth}
%\includegraphics[width=3.0cm,height=3.0cm]{figures/c13-90gpa-jcis.pdf}
\begin{tikzpicture}
\node at (0,0){\includegraphics[width=3.0cm,height=3.0cm]{figures/c13-90gpa-jcis.pdf}};
\draw[] node at (2,0){\bf c13};
\end{tikzpicture}
\label{dmc_c13}
\end{subfigure}

\hspace{-1.0cm}
\begin{subfigure}{0.17\textwidth}
\includegraphics[width=3.0cm,height=3.0cm]{figures/c14-90gpa-hf.pdf}
\label{hf_c14}
\end{subfigure}
\begin{subfigure}{0.17\textwidth}
\includegraphics[width=3.0cm,height=3.0cm]{figures/c14-90gpa-jcsf.pdf}
\label{vmc_c14}
\end{subfigure}
\begin{subfigure}{0.17\textwidth}
\includegraphics[width=3.0cm,height=3.0cm]{figures/c14-90gpa-tddft.pdf}
\label{pbe0_c14}
\end{subfigure}
\begin{subfigure}{0.17\textwidth}
\includegraphics[width=3.0cm,height=3.0cm]{figures/c14-90gpa-bse.pdf}
\label{bse_c14}
\end{subfigure}
\begin{subfigure}{0.17\textwidth}
\includegraphics[width=3.0cm,height=3.0cm]{figures/c14-90gpa-cis.pdf}
\label{cis_c14}
\end{subfigure}
\begin{subfigure}{0.17\textwidth}
%\includegraphics[width=3.0cm,height=3.0cm]{figures/c14-90gpa-jcis.pdf}
\begin{tikzpicture}
\node at (0,0){\includegraphics[width=3.0cm,height=3.0cm]{figures/c14-90gpa-jcis.pdf}};
\draw[] node at (2,0){\bf c14};
\end{tikzpicture}
\label{dmc_c14}
\end{subfigure}

\hspace{-1.0cm}
\begin{subfigure}{0.17\textwidth}
\includegraphics[width=3.0cm,height=3.0cm]{figures/c15-90gpa-hf.pdf}
\label{hf_c15}
\end{subfigure}
\begin{subfigure}{0.17\textwidth}
\includegraphics[width=3.0cm,height=3.0cm]{figures/c15-90gpa-jcsf.pdf}
\label{vmc_c15}
\end{subfigure}
\begin{subfigure}{0.17\textwidth}
\includegraphics[width=3.0cm,height=3.0cm]{figures/c15-90gpa-tddft.pdf}
\label{pbe0_c15}
\end{subfigure}
\begin{subfigure}{0.17\textwidth}
\includegraphics[width=3.0cm,height=3.0cm]{figures/c15-90gpa-bse.pdf}
\label{bse_c15}
\end{subfigure}
\begin{subfigure}{0.17\textwidth}
\includegraphics[width=3.0cm,height=3.0cm]{figures/c15-90gpa-cis.pdf}
\label{cis_c15}
\end{subfigure}
\begin{subfigure}{0.17\textwidth}
%\includegraphics[width=3.0cm,height=3.0cm]{figures/c15-90gpa-jcis.pdf}
\begin{tikzpicture}
\node at (0,0){\includegraphics[width=3.0cm,height=3.0cm]{figures/c15-90gpa-jcis.pdf}};
\draw[] node at (2,0){\bf c15};
\end{tikzpicture}
\label{dmc_c15}
\end{subfigure}

\caption{Excitation-induced density difference, $\Delta\rho({\bf r})$, for
nuclear configurations {\bf c11}--{\bf c15} at $\rho/\rho_0=8.48$.
}
\label{fig:drho-c11-c15}
\end{figure*}

% 90gpa 16-20 %%%%%%%%%%%%%%%%%%%%%%%%%%%%%%%%%%%%%%%%%%%%%%%%%%%%%%%%%%%%%%%%%%%%%%%%%%%%%%%%%%

\begin{figure*}[h]

\hspace{-1.0cm}
\begin{subfigure}{0.17\textwidth}
\captionsetup{labelformat=empty}
\caption{{\em 1CSF0}}
\includegraphics[width=3.0cm,height=3.0cm]{figures/c16-90gpa-hf.pdf}
\label{hf_c16}
\end{subfigure}
\begin{subfigure}{0.17\textwidth}
\captionsetup{labelformat=empty}
\caption{DMC {\em J1CSF}}
\includegraphics[width=3.0cm,height=3.0cm]{figures/c16-90gpa-jcsf.pdf}
\label{vmc_c16}
\end{subfigure}
\begin{subfigure}{0.17\textwidth}
\captionsetup{labelformat=empty}
\caption{TDDFT}
\includegraphics[width=3.0cm,height=3.0cm]{figures/c16-90gpa-tddft.pdf}
\label{pbe0_c16}
\end{subfigure}
\begin{subfigure}{0.17\textwidth}
\captionsetup{labelformat=empty}
\caption{BSE}
\includegraphics[width=3.0cm,height=3.0cm]{figures/c16-90gpa-bse.pdf}
\label{bse_c16}
\end{subfigure}
\begin{subfigure}{0.17\textwidth}
\captionsetup{labelformat=empty}
\caption{{\em CIS0}}
\includegraphics[width=3.0cm,height=3.0cm]{figures/c16-90gpa-cis.pdf}
\label{cis_c16}
\end{subfigure}
\begin{subfigure}{0.17\textwidth}
\captionsetup{labelformat=empty}
\caption{DMC {\em JCIS}}
%\includegraphics[width=3.0cm,height=3.0cm]{figures/c16-90gpa-jcis.pdf}
\begin{tikzpicture}
\node at (0,0){\includegraphics[width=3.0cm,height=3.0cm]{figures/c16-90gpa-jcis.pdf}};
\draw[] node at (2,0){\bf c16};
\end{tikzpicture}
\label{dmc_c16}
\end{subfigure}

\hspace{-1.0cm}
\begin{subfigure}{0.17\textwidth}
\includegraphics[width=3.0cm,height=3.0cm]{figures/c17-90gpa-hf.pdf}
\label{hf_c17}
\end{subfigure}
\begin{subfigure}{0.17\textwidth}
\includegraphics[width=3.0cm,height=3.0cm]{figures/c17-90gpa-jcsf.pdf}
\label{vmc_c17}
\end{subfigure}
\begin{subfigure}{0.17\textwidth}
\includegraphics[width=3.0cm,height=3.0cm]{figures/c17-90gpa-tddft.pdf}
\label{pbe0_c17}
\end{subfigure}
\begin{subfigure}{0.17\textwidth}
\includegraphics[width=3.0cm,height=3.0cm]{figures/c17-90gpa-bse.pdf}
\label{bse_c17}
\end{subfigure}
\begin{subfigure}{0.17\textwidth}
\includegraphics[width=3.0cm,height=3.0cm]{figures/c17-90gpa-cis.pdf}
\label{cis_c17}
\end{subfigure}
\begin{subfigure}{0.17\textwidth}
%\includegraphics[width=3.0cm,height=3.0cm]{figures/c17-90gpa-jcis.pdf}
\begin{tikzpicture}
\node at (0,0){\includegraphics[width=3.0cm,height=3.0cm]{figures/c17-90gpa-jcis.pdf}};
\draw[] node at (2,0){\bf c17};
\end{tikzpicture}
\label{dmc_c17}
\end{subfigure}

\hspace{-1.0cm}
\begin{subfigure}{0.17\textwidth}
\includegraphics[width=3.0cm,height=3.0cm]{figures/c18-90gpa-hf.pdf}
\label{hf_c18}
\end{subfigure}
\begin{subfigure}{0.17\textwidth}
\includegraphics[width=3.0cm,height=3.0cm]{figures/c18-90gpa-jcsf.pdf}
\label{vmc_c18}
\end{subfigure}
\begin{subfigure}{0.17\textwidth}
\includegraphics[width=3.0cm,height=3.0cm]{figures/c18-90gpa-tddft.pdf}
\label{pbe0_c18}
\end{subfigure}
\begin{subfigure}{0.17\textwidth}
\includegraphics[width=3.0cm,height=3.0cm]{figures/c18-90gpa-bse.pdf}
\label{bse_c18}
\end{subfigure}
\begin{subfigure}{0.17\textwidth}
\includegraphics[width=3.0cm,height=3.0cm]{figures/c18-90gpa-cis.pdf}
\label{cis_c18}
\end{subfigure}
\begin{subfigure}{0.17\textwidth}
%\includegraphics[width=3.0cm,height=3.0cm]{figures/c18-90gpa-jcis.pdf}
\begin{tikzpicture}
\node at (0,0){\includegraphics[width=3.0cm,height=3.0cm]{figures/c18-90gpa-jcis.pdf}};
\draw[] node at (2,0){\bf c18};
\end{tikzpicture}
\label{dmc_c18}
\end{subfigure}

\hspace{-1.0cm}
\begin{subfigure}{0.17\textwidth}
\includegraphics[width=3.0cm,height=3.0cm]{figures/c19-90gpa-hf.pdf}
\label{hf_c19}
\end{subfigure}
\begin{subfigure}{0.17\textwidth}
\includegraphics[width=3.0cm,height=3.0cm]{figures/c19-90gpa-jcsf.pdf}
\label{vmc_c19}
\end{subfigure}
\begin{subfigure}{0.17\textwidth}
\includegraphics[width=3.0cm,height=3.0cm]{figures/c19-90gpa-tddft.pdf}
\label{pbe0_c19}
\end{subfigure}
\begin{subfigure}{0.17\textwidth}
\includegraphics[width=3.0cm,height=3.0cm]{figures/c19-90gpa-bse.pdf}
\label{bse_c19}
\end{subfigure}
\begin{subfigure}{0.17\textwidth}
\includegraphics[width=3.0cm,height=3.0cm]{figures/c19-90gpa-cis.pdf}
\label{cis_c19}
\end{subfigure}
\begin{subfigure}{0.17\textwidth}
%\includegraphics[width=3.0cm,height=3.0cm]{figures/c19-90gpa-jcis.pdf}
\begin{tikzpicture}
\node at (0,0){\includegraphics[width=3.0cm,height=3.0cm]{figures/c19-90gpa-jcis.pdf}};
\draw[] node at (2,0){\bf c19};
\end{tikzpicture}
\label{dmc_c19}
\end{subfigure}

%\hspace{-1.0cm}
%\begin{subfigure}{0.17\textwidth}
%\includegraphics[width=3.0cm,height=3.0cm]{figures/c20-90gpa-hf.pdf}
%\label{hf_c20}
%\end{subfigure}
%\begin{subfigure}{0.17\textwidth}
%\includegraphics[width=3.0cm,height=3.0cm]{figures/c20-90gpa-jcsf.pdf}
%\label{vmc_c20}
%\end{subfigure}
%\begin{subfigure}{0.17\textwidth}
%\includegraphics[width=3.0cm,height=3.0cm]{figures/c20-90gpa-tddft.pdf}
%\label{pbe0_c20}
%\end{subfigure}
%\begin{subfigure}{0.17\textwidth}
%\includegraphics[width=3.0cm,height=3.0cm]{figures/c20-90gpa-bse.pdf}
%\label{bse_c20}
%\end{subfigure}
%\begin{subfigure}{0.17\textwidth}
%\includegraphics[width=3.0cm,height=3.0cm]{figures/c20-90gpa-cis.pdf}
%\label{cis_c20}
%\end{subfigure}
%\begin{subfigure}{0.17\textwidth}
%%\includegraphics[width=3.0cm,height=3.0cm]{figures/c20-90gpa-jcis.pdf}
%\begin{tikzpicture}
%\node at (0,0){\includegraphics[width=3.0cm,height=3.0cm]{figures/c20-90gpa-jcis.pdf}};
%\draw[] node at (2,0){\bf c20};
%\end{tikzpicture}
%\label{dmc_c20}
%\end{subfigure}

\caption{Excitation-induced density difference, $\Delta\rho({\bf r})$, for
nuclear configurations {\bf c16}--{\bf c19} at $\rho/\rho_0=8.48$.
}
\label{fig:drho-c16-c19}
\end{figure*}


\begin{figure}
\includegraphics[width=\columnwidth]{figures/tdm2_sm_5gpa.pdf}
\caption{Square modulus of the Cartesian components of the ground-to-excited-state transition dipole
moment in atomic units, for
$\rho/\rho_0=3.15$, 
obtained with VMC using {\em 1CSF0}, {\em J1CSF}, {\em CIS0} and {\em JCIS}
wave functions.  The statistical errors are smaller than the symbol size.
}
\label{fig:tdma}
\end{figure}


\begin{figure}
\includegraphics[width=\columnwidth]{figures/tdm2_sm_10gpa.pdf}
\caption{Same as Fig.~\ref{fig:tdma} for 
$\rho/\rho_0=4.47$.
}
\label{fig:tdmb}
\end{figure}


\begin{figure}
\includegraphics[width=\columnwidth]{figures/tdm2_sm_90gpa.pdf}
\caption{Same as Fig.~\ref{fig:tdma} for 
$\rho/\rho_0=8.48$.
}
\label{fig:tdmc}
\end{figure}

\begin{table}[h]
\begin{tabular}{|r|l|l|l|l|l|l|}
\hline
$\rho/\rho_0$ & {\em 1CSF0} & {\em J1CSF} & {\em CIS0} & {\em JCIS} & TDDFT & BSE  \\
\hline
3.15  & 0.09(4) & 0.12(5) & 0.75(11) & 0.70(10) & 0.07(3) & 0.36(7) \\
4.47  & 0.05(1) & 0.07(2) & 0.67(7) & 0.64(7) &           & \\
8.48  & 0.06(2) & 0.08(2) & 0.32(8) & 0.33(7) &           & \\
\hline
\end{tabular}
\caption{
Oscillator strength as a function of density averaged over nuclear
configurations, obtained by VMC with various wave functions.
For the lowest density we also list the TDDFT and BSE results for comparison.
}
\label{table:os}
\end{table}


\end{document}
